# Supplementary material for: Data Efficient Human Intention Prediction: Leveraging Neural Network Verification and Expert Guidance
Source: arXiv:2108.06871 source file (2022-09-24)
Supplement: Supplementary file 1 [file C_Qv_D.tex]

% This file was created by tikzplotlib v0.9.3.
\begin{tikzpicture}

\definecolor{color0}{rgb}{0.1,0,0.95}
\definecolor{color1}{rgb}{1,0,0}
\definecolor{color2}{rgb}{1,0.498,0.0549}
\pgfplotsset{compat=1.5}
\begin{groupplot}[group style={group size=2 by 1, horizontal sep=60pt}]
\nextgroupplot[
width = 0.48\linewidth,
height = 4.5cm,
font = \small,%\footnotesize,
legend cell align={left},
legend style={nodes={scale=0.5, transform shape}, fill opacity=0.8, draw opacity=1, text opacity=1, draw=white!80!black},
tick align=inside,
tick pos=left,
xmin=1000, xmax=5000,
xtick style={color=black},
xlabel={Number of Seeds ($C$)},
ylabel={Level of Expansion},
% ymode=log,
% log basis y={10},
ymin=0, ymax=9,
ytick style={color=black}
]
\addplot [thick, color0]
table {%
1000 4
2000 5
5000 5
};
\addlegendentry{2D Classification}

\addplot [thick, color1]
table {%
1000 4
2000 5
5000 6
};
\addlegendentry{Robot Handover}

\addplot [thick, color2]
table {%
1000 1
2000 2
5000 3
};
\addlegendentry{Human Assembly}

\nextgroupplot[
width = 0.48\linewidth,
height = 4.5cm,
font = \small,%\footnotesize,
legend cell align={left},
legend style={nodes={scale=0.5, transform shape}, fill opacity=0.8, draw opacity=1, text opacity=1, draw=white!80!black},
tick align=inside,
tick pos=left,
xmin=1000, xmax=5000,
xtick style={color=black},
xlabel={Number of Seeds ($C$)},
ylabel={Num of Augmented Data},
% ymode=log,
% log basis y={10},
ymin=0, ymax=22000,
ytick={0,10000,20000},
ytick style={color=black}
]
\addplot [thick, color0]
table {%
1000 2974
2000 4446
5000 5281
};
\addlegendentry{2D Classification}

\addplot [thick, color1]
table {%
1000 2997
2000 5962
5000 9468
};
\addlegendentry{Robot Handover}

\addplot [thick, color2]
table {%
1000 6505
2000 11010
5000 21020
};
\addlegendentry{Human Assembly}

\end{groupplot}
\end{tikzpicture}
