# Supplementary material for: Data Efficient Human Intention Prediction: Leveraging Neural Network Verification and Expert Guidance
Source: arXiv:2108.06871 source file (2022-09-24)
Supplement: Supplementary file 3 [file rv_time.tex]

% This file was created by tikzplotlib v0.9.3.
\begin{tikzpicture}

\definecolor{color0}{rgb}{0.1,0,0.95}
\definecolor{color1}{rgb}{1,0,0}
\definecolor{color2}{rgb}{1,0.498,0.0549}
\pgfplotsset{compat=1.5}
\begin{groupplot}[group style={group size=3 by 1}]
\nextgroupplot[
width = \linewidth,
height = 4cm,
font = \small,%\footnotesize,
legend cell align={left},
legend style={nodes={scale=0.6, transform shape}, fill opacity=0.8, draw opacity=1, text opacity=1, draw=white!80!black},
tick align=inside,
tick pos=left,
xmin=0, xmax=1100,
xtick style={color=black},
xlabel={Inner Optimization Frequency ($r$)},
ylabel={Time (s)},
ymode=log,
log basis y={10},
ymin=0, ymax=20000,
ytick style={color=black}
]
\addplot[mark=triangle*,color0]
table {%
50 468.149
500 43.906
1000 39.141
};
\addlegendentry{2D Classification}

\addplot [mark=*, color1]
table {%
50 12895
500 395
1000 131.817
};
\addlegendentry{Robot Handover}

\addplot [mark=square*, color2]
table {%
50 5835.460
500 183.601
1000 94.250
};
\addlegendentry{Human Assembly}

\end{groupplot}
\end{tikzpicture}
